# Supplementary material for: Electric Field Intensity Modulated Scattering as a Thin-Film Depth Probe
Source: arXiv:1907.12217 ancillary file (2019-12-20)
Supplement: Supplementary file 1 [file EFI_SI.pdf]

# Supplementary Information for: Electric Field Intensity Modulated Scattering as a Thin-Film Depth Probe

Peter J. Dudenas[a,b*], Adam Z. Weber[b], and Ahmet Kusoglu[b]

[a]Chemical and Biomolecular Engineering, University of California, Berkeley, CA 94720 USA

[b]Energy Conversion Group, Lawrence Berkeley National Lab, CA 94720 USA

## 1 Electric Field Intensity Calculations

Parrat's recursion[1] is used to calculate the electric field intensity throughout a thin film using equations in *X-Ray Scattering from Soft-Matter Thin Films*[2].These equations are derived for s-polarized x-rays, as typically produced by synchrotron bending magnets and undulators.

A sample is divided into N+1 layers, and the ratio of reflected to transmitted waves is calculated via Equation 1

$$X_j = \frac{R_j}{T_j} = e^{-2ik_{z,j}z_j} \frac{r_{j,j+1} + X_{j+1}e^{2ik_{z,j+1}z_j}}{1 + r_{j,j+1}X_{j+1}e^{2ik_{z,j+1}z_j}} \tag{1}$$

where

$$r_{j,j+1} = \frac{k_{z,j} - k_{z,j+1}}{k_{z,j} + k_{z,j+1}} \qquad k_{z,j} = k\left(n_j^2 - \cos^2\alpha_i\right)^{\frac{1}{2}}$$

$n_j$ is the complex index of refraction in layer j, $\alpha_i$ is the incidence angle, and k is the x-ray wave vector in vacuum. $r_{j,j+1}$ is the Fresnel reflection coefficient at the interface between layers j and j+1. The substrate is assumed to be thick enough such that no reflections occur and $R_{N+1} = 0$. Starting at j=N, $X_j$ is calculated recursively up to layer j = 1, where $T_1$ has been normalized to 1 and so $X_1 = R_1$ is known. $|R_1|^2$ is the specular reflection as measured in traditional x-ray reflectivity experiments.

Using Equations 2 and 3, the complex wave amplitudes through the rest of the film can be calculated

$$R_{j+1} = \frac{1}{t_{j+1,j}}\left[T_j r_{j+1,j} e^{-i(k_{z,j+1}+k_{z,j})z_j} + R_j e^{-i(k_{z,j+1}-k_{z,j})z_j}\right] \tag{2}$$

$$T_{j+1} = \frac{1}{t_{j+1,j}}\left[T_j e^{i(k_{z,j+1}-k_{z,j})z_j} + R_j r_{j+1,j} e^{i(k_{z,j+1}+k_{z,j})z_j}\right] \tag{3}$$

where

$$t_{j+1,j} = 1 + r_{j+1,j}$$

Layer roughness can be incorporated via the Fresnel coefficients or treated as a graded interface with a smoothly varying index of refraction between the two layers.

Once the reflected and transmitted complex wave amplitudes are known for each layer, the electric field intensity (EFI) can be calculated using Equation 4

$$EFI = \left|T^i e^{-ik_z^i z} + R^i e^{ik_z^i z}\right|^2 \tag{4}$$

# 2 7.3.3 Energy Distribution

Beamline 7.3.3 uses a multilayer monochromator to maximize x-ray beam flux from the bending magnet source. This results in a relatively large energy FWHM (Figure S1a), and needs to be accounted for when calculating EFI. This is done by using the above equations to calculate EFI at each energy, and summing, weighted by the PDF. Accordingly, the index of refraction for each layer needs to be adjusted. The Center for X-Ray Optics (CXRO) online calculator provides an excellent tool to estimate how the index of refraction varies for a given material[3]. Figure S1b plots the index of refraction for Nafion and silicon in this energy range

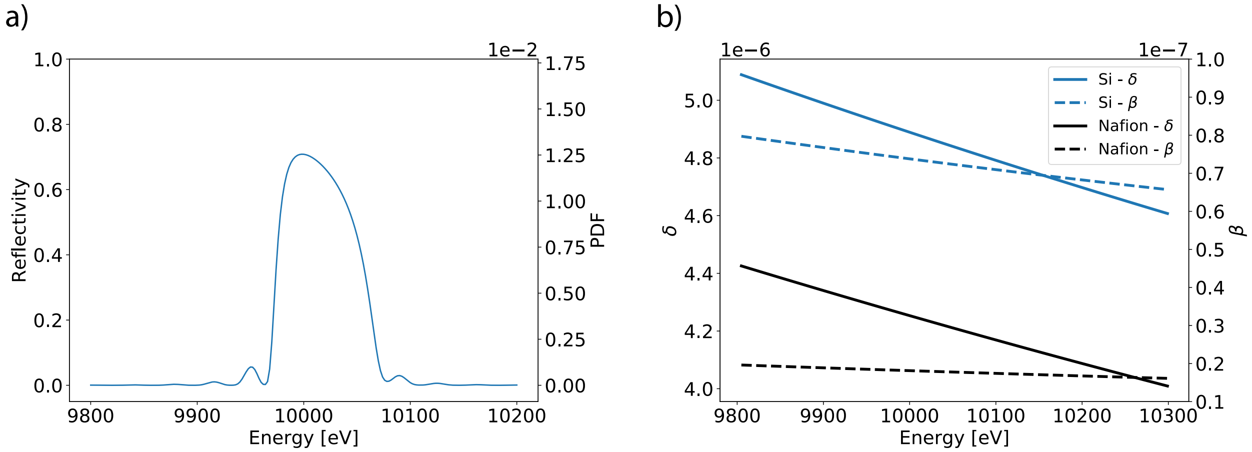


Figure S1: a) Reflectivity and probability distribution function (PDF) plotted versus energy for Beamline 7.3.3 at the Advanced Light Source. b) Real and imaginary parts of the index of refraction for Nafion and silicon versus energy

## 3 Collection Schematic

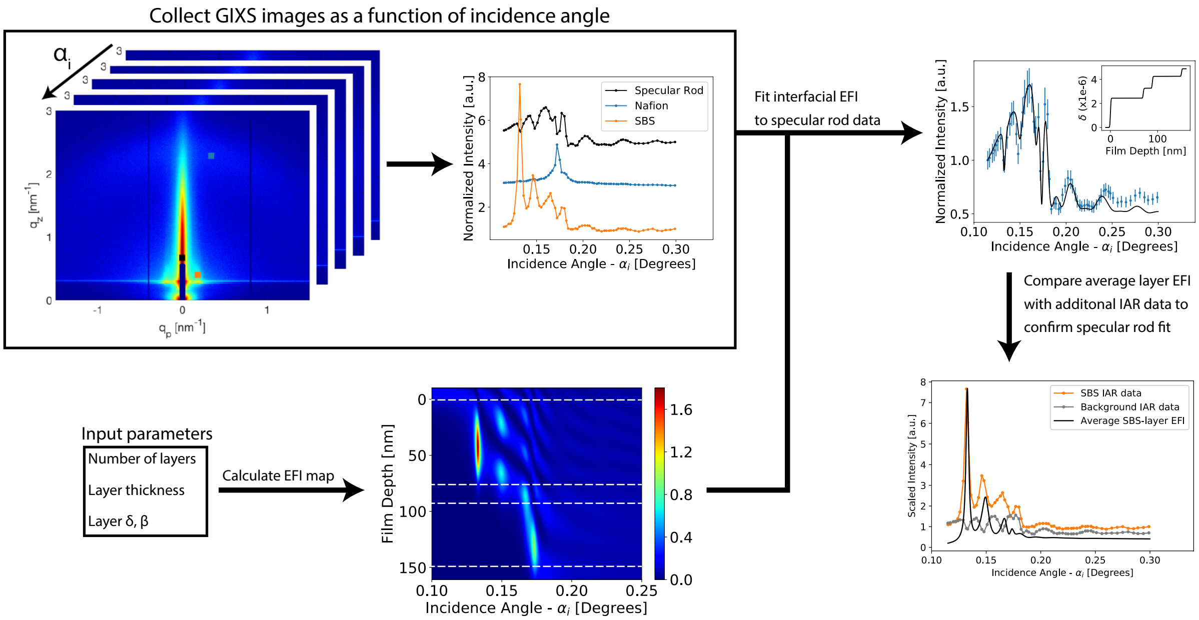


Figure S2: Data collection and analysis procedure

## 4 Bilayer Samples

To confirm that the signal from SBS and Nafion's scattering peaks are indeed coming from their respective layers, the average EFI for that layer is plotted alongside the experimental data (Figure S3).

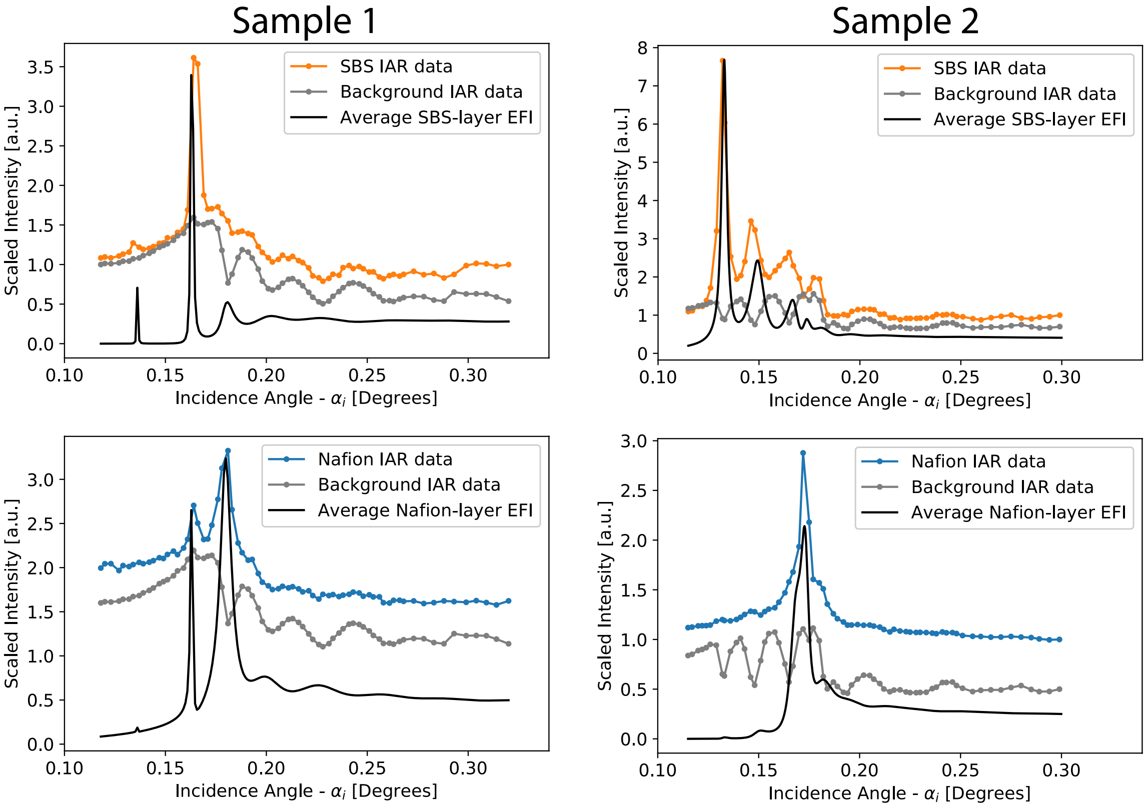


Figure S3: Comparison of Nafion and SBS IAR data with background IAR data and calculated average layer EFI

For both Sample 1 and Sample 2, there is good agreement between the position of the TE modes within each layer which confirms their respective positions within the film. However, since the scattering signal from SBS and Nafion is relatively weak, there is also a contribution from background that scales similarly to the specular rod. Away from the TE modes in each layer, the Nafion and SBS IAR data have similar modulations to the background IAR data. While the specular rod appears as a sharp rod near $q_p$=0, scattering from interfacial roughness extends in $q_p$ and $q_z$ with some non-zero intensity and contributes to observed EFI modulations in weakly scattering signals. While this technique has the potential to elucidate significantly more information from grazing incidence scattering images, various contributions to the observed EFI modulation must carefully accounted for.

## References


[1] L. G. Parratt, "Surface studies of solids by total reflection of x-rays," *Physical Review*, vol. 95, no. 2, pp. 359–369, 1954.

[2] M. Tolan, *X-ray scattering from soft-matter thin films: materials science and basic research*. Springer, 1999.

[3] B. L. Henke, E. M. Gullikson, and J. C. Davis, "X-ray interactions: Photoabsorption, scattering, transmission, and reflection at e = 50-30,000 ev, z = 1-92," *Atomic Data and Nuclear Data Tables*, vol. 54, no. 2, pp. 181–342, 1993.
